# Supplementary material for: Efficient SimRank Computation via Linearization
Source: arXiv:1411.7228 source file (2014-11-26)
Supplement: Supplementary file 3 [file appendix2.tex]

%\clearpage
\appendix

\medskip

In Appendix, we give omitted proofs of propositions in the paper.
We first prove the non probablistic results (i.e, Propositions 1, 2, 4 and 6) and then prove other probablistic results (concentration bounds).

\begin{proof}[of Proposition~\ref{prop:linearizedsimrank}]
Let $S(D)$ be a matrix that satisfies
\begin{align} \label{eq:SD}
  S(D) = c P^\top S(D) P + D.
\end{align}
We first prove that $S(D)$ is well-defined.
Let $\mathrm{vec}: \mathbb{R}^{n \times n} \to \mathbb{R}^{n^2}$ be the vectorization operation
defined by $\mathrm{vec}(A)_{i+nj} = A_{ij}$. Using $\mathrm{vec}$, \eqref{eq:SD} is written as
the linear equation
\begin{align} \label{eq:sylvester}
  \left( I - c P^\top \otimes P^\top \right) \mathrm{vec}(S(D)) = \mathrm{vec}(D).
\end{align}
Since the coefficient matrix of \eqref{eq:sylvester} is nonsingular, it a unique solution.
This proves the well-definedness of $S(D)$.

Next, we prove that $D$ is uniquely determined under the condition $S(D)_{ii} = 1$ for all $i \in V$.
Write this condition by using \eqref{eq:sylvester} with a partitioned system:
\[
\begin{bmatrix} I - c P_{DD} & - P_{DO}\\ - P_{OD} & I - c P_{OO} \end{bmatrix} \begin{bmatrix} \vec{1} \\ u \end{bmatrix} = \begin{bmatrix} d \\ 0 \end{bmatrix},
\]
where $d$ denotes diagonal entries of $D$ and $u$ be an arbitrary vector.
We observe that we can eliminate $u$ from this equation.
The eliminated system is
\[
  d= \left( (I - c P_{DD}) - c^2 P_{DD} (I - c P_{OO})^{-1} P_{OD} \right) \vec{1}.
\]
Since this formula does not depend on $u$,
$D$ is uniquely determined by the diagonal condition of $S(D)$.
Note that the above gives an explicit formula of $D$. 
\end{proof}

\begin{proof}[of Proposition~\ref{prop:dbound}]
Since $D$ satisfies
%\[
$
  D = S - c P^\top S P
$,
%\]
we have
\[
  D_{uu} = 1 - c (P e_u)^\top S P e_u.
\]
Since $P e_u$ is a stochastic vector, we have
\[
  1 - c \max_{ij} S_{ij} \le D_{uu} \le 1 - c \min_{ij} S_{ij}
\]
By the random surfer pair interpretation of SimRank, we have $0 \le S_{ij} \le 1$.
Therefore we obtain
  $1 - c \le D_{uu} \le 1$. 
\end{proof}
\begin{proof}[of Proposition~\ref{prop:L1bound}]
Consider %the $t$-th term of \eqref{eq:expansionuv}, i.e.,
$ (P^t e_u)^\top D (P^t e_v)$.
Since $P^t e_v$ is a stochastic vector, by \eqref{eq:l1}, we have
\begin{align} \label{eq:tthbound}
  (P^t e_u)^\top D (P^t e_v) \le \max_{w \in \mathrm{supp}(P^t e_v)} (P^t e_u)^\top D e_w,
\end{align}
Since $P^t e_v$ corresponds to a $t$-step random walk,
the support is contained by a ball of radius $t$ centered at $v$.
Therefore we have
\begin{align*}
  (P^t e_u)^\top D (P^t e_v) \le \max_{w \in V : d-t \le d(u, w) \le d+t} (P^t e_u)^\top D e_w
\end{align*}
By plugging \eqref{eq:alpha}, we have
\[
  (P^t e_u)^\top D (P^t e_v) \le \max_{d - t \le d' \le d + t} \alpha(u, d', t).
\]
Substitute the above to \eqref{eq:expansionuv},
we obtain \eqref{eq:upperbound1}. 
\end{proof}
\begin{proof}[of Proposition~\ref{prop:L2bound}]
Consider %the $t$-th term of \eqref{eq:expansionuv}, i.e.,
$ c^t (P^t e_u)^\top D (P^t e_v)$.
By \eqref{eq:l2},  we have
\[
  (P^t e_u)^\top D (P^t e_v) = (\sqrt{D} P^t e_u)^\top  (\sqrt{D} P^t e_v) \le \gamma(u,t) \gamma(v,t).
\]
Substitute the above to \eqref{eq:expansionuv},
we obtain \eqref{eq:upperbound2}. 
\end{proof}

Let us start the proof of concentration bounds.
We first prepare some basic probablistic inequalities.
\begin{lemma}[Hoeffding's inequality]
  Let $X_1, \ldots, X_R$ be independent random variables with $X_r \in [0,1]$ for all $r = 1, \ldots, R$.
Let $S := (X_1 + \cdots + X_R)/R$.  Then
\[
  \P\left\{ \left| S - \E[S] \right| \ge \epsilon \right\} \le 2 \exp(-2 \epsilon^2 R).
\]
\end{lemma}
%In the rest of the proofs for some propositions, we need the following variant of
%Hoeffding's inequality.
%We need two ``max'' variants of Hoeffding's inequality.
\begin{lemma}[Max-Hoeffding's inequality] \label{lem:hoeffding2}
For each $f = 1, \ldots, F$, let $X_r(f)$ ($r = 1, \ldots, R$) be independent random variables with $X_r(f) \in [0,1]$.
Let $S(f) := (X_1(f) + \cdots + X_R(f))/R$.  Then
\[
  \P\left\{ \max_f \left| S(f) - \E[S(f)] \right| \ge \epsilon \right\} \le 2 F \exp(-2 \epsilon^2 R).
\]
\end{lemma}
\begin{proof}
\begin{align*}
& \P\left\{ \max_f \left| S(f) - \E[S(f)] \right| \ge \epsilon \right\}  \\
%&\le \P\left\{ \bigcup_{f} \left\{ \left| S(f) - \E[S(f)] \right| \ge \epsilon \right\} \right\}  \\
&\le \sum_f \P\left\{ \left| S(f) - \E[S(f)] \right| \ge \epsilon \right\} \le 2 F \exp(-2 \epsilon^2 R). 
\end{align*}
\end{proof}
%\begin{lemma} \label{lem:hoeffding3}
%For each $f = 1, \ldots, F$, let $X_r(f)$ ($r = 1, \ldots, R$) be independent random variables with $X_r(f) \in [0,1]$.
%Let $S(f) := (X_1(f) + \cdots + X_R(f))/R$.  Then
%\[
%  \P\left\{ \left| \max_f S(f) - \max_f \E[S(f)] \right| \ge \epsilon \right\} \le (F+1) \exp(-2 \epsilon^2 R).
%\]
%\end{lemma}
%\begin{proof}
%\begin{align*}
%  & \P\left\{ \max_f S(f) - \max_f \E[S(f)]  \ge \epsilon \right\} \\
%  &= \P\left\{ \bigcup_f \left\{ S(f) - \max_f \E[S(f)]\ge \epsilon \right\} \right\} \\
%  &\le \sum_f \P\left\{ S(f) - \max_f \E[S(f)]\ge \epsilon \right\} \\
%  &\le \sum_f \P\left\{ S(f) - \E[S(f)] \ge \epsilon + \max_f \E[S(f)]- \E[S(f)] \right\}  \\
%  &\le \sum_f \P\left\{ S(f) - \E[S(f)] \ge \epsilon  \right\} \le F \exp(-2 \epsilon^2 R).
%\end{align*}
%Let $f^* = \arg\max \E[S(f)]$. Then
%\begin{align*}
%  & \P\left\{ \max_f \E[S(f)] - \max_f S(f) \ge \epsilon \right\} \\
%  &\le \P\left\{ \max_f \E[S(f)] - S(f^*) \ge \epsilon \right\} \le \exp(-2 \epsilon^2 R).
%\end{align*}
%Therefore
%\begin{align*}
% \P\left\{ \left| \max_f S(f) - \max_f \E[S(f)] \right|  \ge \epsilon \right\}
%\le (F+1) \exp(-2 \epsilon^2 R).
%\end{align*}
%\end{proof}

We write
$u_r^{(t)}$ and $v_r^{(t)}$ ($r = 1, \ldots, R$) for the $t$-th positions of independent random walks start from $u$ and $v$ and follow the in-links, respectively,
and $X_u^{(t)} := (1 / R) \sum_{r=1}^R e_{u_r^{(t)}}$, $X_v^{(t)} := (1 / R) \sum_{r=1}^R e_{v_r^{(t)}}$.

%\begin{lemma} \label{lem:Pubound}
%\begin{align}
%  \P\left\{ \left| X_u^{(t)} - P^t e_u \right|_{\infty} \ge \epsilon \right\} \le (n+1) \exp(- 2 \epsilon^2 R).
%\end{align}
%\end{lemma}
%\begin{proof}
%This is a direct application of Lemma~\ref{lem:hoeffding2}.
%\end{proof}
\begin{lemma} \label{lem:Dbound}
For each $w \in V$,
\begin{align*}
  \P\left\{ \left| X_u^{(t)\top} D e_w - (P^t e_u)^\top D e_w \right| \ge \epsilon \right\} \le 2 \exp(- 2 \epsilon^2 R).
\end{align*}
\end{lemma}
\begin{proof}
\begin{align*}
  & \P\left\{ \left| X_u^{(t) \top} D e_w - (P^t e_u)^\top D e_w \right| \ge \epsilon \right\} \\
  &\le \P\left\{ \left| X_u^{(t)^\top} e_w - (P^t e_u)^\top e_w \right| \ge \epsilon \right\}
  \le 2 \exp(-2 \epsilon^2 R). 
\end{align*}
\end{proof}

\begin{lemma} \label{lem:Duvbound}
\begin{align*}
  \P\left\{ \left| X_u^{(t) \top} D X_v^{(t)} - (P^t e_u)^\top D P^t e_v \right| \ge \epsilon \right\}
  \le 4 n \exp(- \epsilon^2 R / 2).
\end{align*}
\end{lemma}
\begin{proof}
\begin{align*}
& \P\left\{ \left| X_u^{(t) \top} D X_v^{(t)} - (P^t e_u)^\top D P^t e_v \right| \ge \epsilon \right\} \\
&\le \P \left\{ \left| X_u^{(t) \top} D \left( X_v^{(t)} - P^t e_v \right) \right| \ge \epsilon/2 \right\} \\
&+ \P \left\{ \left| \left( X_u^{(t)} - P^t e_u\right)^\top D P^t e_v \right| \ge \epsilon/2 \right\} \\
&\le 4 n \exp(-\epsilon^2 R / 2). 
\end{align*}
\end{proof}

\begin{proof}[of Proposition~\ref{prop:bound}]
By Lemma~\ref{lem:Duvbound}, we have
\begin{align*}
  & \P \left\{ \left| \left( \sum_{t=0}^{T-1} c^t X_u^{(t) \top} D X_v^{(t)} \right) - s^{(T)}(u,v) \right| \ge \epsilon \right\} \\
  \le & \sum_{t = 0}^{T-1} \P \left\{ \left| c^t X_u^{(t) \top} D X_v^{(t)} - c^t (P^t e_u)^\top D P^t e_v \right| \ge c^t \epsilon/(1-c)\right\} \\
  \le & 4 n T \exp \left( - \epsilon^2 R / 2(1-c)^2\right). 
\end{align*}
\end{proof}

\begin{proof}[of Proposition~\ref{prop:L1sample}]
We first prove the bound of $\alpha(u,d,t)$.
%Consider random walks $u^{(t)}_r$ ($r = 1, \ldots, R$).
%Then
Note that
$\alpha(u,d,t) = \max_{w} \{ P^t e_u D e_w \}$
and the algorithm computes
$\tilde \alpha(u,d,t) = \max_{w} \{ X_u^{(t) \top} D e_w \}.$
By Lemmas~\ref{lem:Dbound} and \ref{lem:hoeffding2},
we have
\begin{align*}
&\P\left\{ \left| \max_w X_u^{(t) \top} D e_w - \max_w (P^t e_u)^\top D e_w \right| \ge \epsilon \right\} \\
&\le \P\left\{ \max_w \left| X_u^{(t) \top} D e_w - (P^t e_u)^\top D e_w \right| \ge \epsilon \right\} \\
& \le 2n \exp(-2 \epsilon^2 R).
\end{align*}
Using the above estimation, we bound $\beta$ as
\begin{align*}
  & \P\left\{ \left| \tilde \beta(u,d) - \beta(u,d) \right| \ge \epsilon \right\} \\
%  & \le \P\left\{ \bigcup_{d,t} \left\{ |\tilde \alpha(u,d,t) - \alpha(u,d,t)| \ge \epsilon \right\} \right\} \\
  & \le \sum_{d,t} \P\left\{ |\tilde \alpha(u,d,t) - \alpha(u,d,t)| \ge \epsilon \right\} \\
  & \le 2 n d_{\mathrm{max}} T \exp(- 2 \epsilon^2 R). 
\end{align*}
\end{proof}

%\begin{proof}[of Proposition~\ref{prop:L1sample}]
%We first prove the bound of $\alpha(u,d,t)$.
%Consider random walks $u^{(t)}_r$ ($r = 1, \ldots, R$).
%Then
%\[
%  \alpha(u,d,t) = \max_{w} \{ \E[ D_{u^{(t)} w} ] \}
%\]
%and the algorithm computes
%\[
%  \tilde \alpha(u,d,t) = \max_{w} \{ \frac{1}{R} \sum_{r=1}^R D_{u_r^{(t)} w} \}.
%\]
%Therefore, by Lemma~\ref{lem:hoeffding3}, we have
%\[
%  \P\left\{ |\tilde \alpha(u,d,t) - \alpha(u,d,t)| \ge \epsilon \right\} \le 2 T n (n+1) \exp(- 2 R \epsilon^2). 
%\]
%Using the above estimation, we bound $\beta$ as
%\begin{align*}
%  & \P\left\{ \left| \tilde \beta(u,d) - \beta(u,d) \right| \ge \epsilon \right\} \\
%  & \le \P\left\{ \bigcup_{d,t} \left\{ |\tilde \alpha(u,d,t) - \alpha(u,d,t)| \ge \epsilon \right\} \right\} \\
%  & \le \sum_{d,t} \P\left\{ |\tilde \alpha(u,d,t) - \alpha(u,d,t)| \ge \epsilon \right\} \le 2 d_{\mathrm{max}} T^2 n(n+1) (n \exp(-R^2 \epsilon^2).
%\end{align*}
%\end{proof}
%
\begin{proof}[of Proposition~\ref{prop:L2sample}]
We first observe that $\gamma(u,t)^2 = (P^t e_u)^\top D (P^t e_u)$
and the algorithm estimates this value by
\[
  (\tilde \gamma(u,t))^2 = \frac{1}{R^2} D_{u_r^{(t)} u_r^{(t)}}.
\]
Hence, by the same proof as Lemma~\ref{lem:Duvbound}, we have
\[
  \P\left\{ |\tilde \gamma(u,t)^2 - \gamma(u,t)^2| \ge \epsilon \right\} \le 4 n \exp(- \epsilon^2 R/2).
\]
Therefore
\begin{align*}
  & \P\left\{ | \tilde \gamma(u,t) - \gamma(u,t) | \ge \epsilon \right\} \\
  & \le \P\left\{ |\tilde \gamma(u,t)^2 - \gamma(u,t)^2| \ge \frac{\epsilon}{\tilde \gamma(u,t) + \gamma(u,t)} \right\} \\
  & \le \P\left\{ |\tilde \gamma(u,t)^2 - \gamma(u,t)^2| \ge \epsilon/2 \right\} \le 4 n \exp(- \epsilon^2 R / 8).
\end{align*}
Here we use the fact that both $\tilde \gamma(u,t)$ and $\gamma(u,t)$ are smaller than $\sqrt{ \max_w D_{ww} } = 1$. 
\end{proof}
